# Supplementary material for: Scan2Part: Fine-grained and Hierarchical Part-level Understanding of Real-World 3D Scans
Source: arXiv:2206.02366 source file (2022-06-06)
Supplement: Supplementary file 3 [file 03_results.tex]

\section{Detailed segmentation results}
\label{supsec:segmentation-detail}

% \paragraph{Specifications of our benchmarked networks. }
% \label{supsec:results:network-detail}

\subsection{Part-level semantic labeling}
\label{supsec:results:semantic-segmentation}

Please see more part-level semantic labeling results in Tables~\ref{suptbl:partseg-iou}--

% \AN{3 tables with class-wise results on part semantic segmentation for 3 different levels of detail}

\begin{table}[!h]
\caption{Coarse level mean IoU (\%)}
\centering
\begin{tabular}{lrrrrrrrr}
\toprule
 &  \multicolumn{2}{c}{Baseline} && \multicolumn{5}{c}{Multi-Task Training (MTT)} \\
 \cmidrule{2-3}
 \cmidrule{5-9}
Class 			  &  	 Coa. &  				Fin. &&  	12 &  		123-coa. &  		123-coa.\,ens. &  	  123-fin. &  123-fin.\,ens. \\
\midrule
Microwave         &       2.0 &                  6.7 &&     5.3 &             4.7 &                     5.8 &           8.0 &                   8.3 \\
Display           &      42.3 &                 28.9 &&    35.7 &            39.9 &                    39.5 &          39.0 &                  39.1 \\
Lamp              &      17.1 &                 11.4 &&    14.0 &            16.5 &                    13.7 &           9.6 &                   8.7 \\
Laptop            &       9.8 &                  5.6 &&     3.4 &            11.9 &                    10.4 &           6.9 &                   6.4 \\
Bag               &      10.0 &                  4.6 &&     6.8 &             7.4 &                     6.6 &           6.0 &                   6.1 \\
Storage\_furniture &      47.2 &                 40.6 &&    42.1 &            56.0 &                    55.3 &          44.3 &                  43.9 \\
Bed               &      32.0 &                 22.1 &&    36.9 &            32.7 &                    33.5 &          32.8 &                  33.2 \\
Table             &      49.2 &                 38.9 &&    47.4 &            46.1 &                    44.4 &          47.7 &                  46.6 \\
Chair             &      55.1 &                 50.3 &&    58.4 &            54.1 &                    53.7 &          62.0 &                  61.8 \\
Dishwasher        &       0.0 &                  0.2 &&     0.0 &             0.3 &                     0.2 &           0.0 &                   0.0 \\
Trash\_can         &      21.3 &                 18.8 &&    30.3 &            18.5 &                    19.3 &          25.8 &                  24.9 \\
Pot               &       1.8 &                  1.0 &&     1.7 &             2.7 &                     3.0 &           1.0 &                   1.1 \\
Keyboard          &       4.1 &                  1.2 &&     0.4 &            11.7 &                    10.8 &           1.3 &                   1.4 \\
\midrule
Mean              &      22.5 &                 17.7 &&    21.7 &            23.3 &                    22.8 &          21.9 &                  21.7 \\
\bottomrule
\end{tabular}
\label{suptbl:partseg-iou}
\end{table}

\begin{table}[!h]

\caption{Coarse level mAcc}
\centering
\begin{tabular}{lrrrrrrrr}
\toprule
 &  \multicolumn{2}{c}{Baseline} && \multicolumn{5}{c}{Multi-Task Training (MTT)} \\
 \cmidrule{2-3}
 \cmidrule{5-9}
Class 			  &  	 Coa. &  				Fin. &&  	12 &  		123-coa. &  		123-coa.\,ens. &  	  123-fin. &  123-fin.\,ens. \\
\midrule
Microwave         &       2.1 &                  9.7 &&     6.9 &             6.1 &                     8.4 &          11.6 &                  13.4 \\
Display           &      66.7 &                 56.0 &&    68.0 &            57.7 &                    58.7 &          67.7 &                  70.2 \\
Lamp              &      41.7 &                 55.3 &&    55.4 &            42.5 &                    44.7 &          48.5 &                  50.5 \\
Laptop            &      13.1 &                 16.8 &&     6.9 &            17.0 &                    17.6 &          11.3 &                  11.5 \\
Bag               &      41.4 &                 40.4 &&    40.3 &            46.1 &                    46.9 &          53.8 &                  53.8 \\
Storage\_furniture &      51.9 &                 44.3 &&    45.1 &            65.8 &                    64.4 &          48.5 &                  48.2 \\
Bed               &      50.1 &                 39.3 &&    56.6 &            50.2 &                    50.7 &          66.5 &                  63.6 \\
Table             &      74.3 &                 52.8 &&    67.7 &            71.7 &                    65.2 &          72.0 &                  67.6 \\
Chair             &      81.0 &                 86.7 &&    90.0 &            67.4 &                    73.0 &          70.7 &                  76.3 \\
Dishwasher        &       0.0 &                  0.3 &&     0.0 &             0.6 &                     0.5 &           0.0 &                   0.0 \\
Trash\_can         &      24.9 &                 21.9 &&    38.9 &            19.5 &                    21.5 &          31.9 &                  33.3 \\
Pot               &       8.6 &                  6.3 &&     8.2 &             7.9 &                     8.0 &           5.4 &                   5.6 \\
Keyboard          &       6.7 &                  4.2 &&     0.6 &            16.2 &                    18.8 &           2.8 &                   3.4 \\
\midrule
Mean              &      62.6 &                 54.2 &&    61.6 &            63.5 &                    62.8 &          60.7 &                  60.5 \\
\bottomrule
\end{tabular}
\end{table}

\begin{table}[!h]

\caption{middle level mIoU}
\centering
\begin{tabular}{lrrrrrrrr}
\toprule
 &  \multicolumn{2}{c}{Baseline} && \multicolumn{5}{c}{Multi-Task Training (MTT)} \\
 \cmidrule{2-3}
 \cmidrule{5-9}
Class 			  &  	 Mid. &  				Fin. &&  	12 &  		123-coa. &  		123-coa.\,ens. &  	  123-fin. &  123-fin.\,ens. \\
\midrule
Microwave/body           &              1.8 &                  6.7 &&     5.4 &             5.2 &                     5.9 &           8.1 &                   8.4 \\
Laptop/screen\_side       &             15.6 &                  9.2 &&     4.7 &            18.3 &                    16.1 &          10.2 &                  10.1 \\
Bag/luggage              &              4.1 &                  0.0 &&     0.5 &             0.0 &                     0.0 &           0.0 &                   0.0 \\
StorageFurniture/cabinet &             44.1 &                 40.2 &&    40.9 &            54.5 &                    55.0 &          40.9 &                  42.6 \\
Bed/regular\_bed          &             38.2 &                 22.0 &&    34.8 &            30.4 &                    33.1 &          31.3 &                  33.3 \\
Table/desk               &              9.2 &                  4.4 &&     7.0 &             5.2 &                     4.7 &           7.8 &                   8.1 \\
Table/regular\_table      &             49.9 &                 39.3 &&    47.3 &            44.0 &                    43.6 &          45.3 &                  45.2 \\
Chair/chair\_base         &             58.0 &                 45.9 &&    53.7 &            45.9 &                    41.8 &          54.2 &                  48.4 \\
Lamp/table\_lamp          &              1.9 &                  5.3 &&    14.4 &             3.7 &                     5.4 &           2.9 &                   4.5 \\
Dishwasher/body          &              0.0 &                  0.2 &&     0.0 &             0.2 &                     0.2 &           0.0 &                   0.0 \\
TrashCan/outside\_frame   &              0.0 &                  0.0 &&     1.4 &             0.0 &                     0.0 &           0.0 &                   0.0 \\
Chair/chair\_arm          &             18.9 &                 11.2 &&    13.0 &            12.7 &                    11.7 &          17.5 &                  15.9 \\
Bed/bunk\_bed             &              2.2 &                  0.9 &&    13.8 &             1.2 &                     1.9 &           1.5 &                   1.9 \\
Chair/chair\_seat         &             50.5 &                 36.9 &&    50.2 &            43.6 &                    38.6 &          47.6 &                  44.1 \\
TrashCan/container       &             34.2 &                 21.7 &&    30.9 &            21.2 &                    21.1 &          28.4 &                  28.7 \\
Vase/containing\_things   &              0.9 &                  1.5 &&     2.1 &             3.3 &                     3.9 &           1.0 &                   1.2 \\
Bag/hand\_or\_shoulder\_bag &              2.6 &                  1.3 &&     1.9 &             2.3 &                     2.2 &           2.0 &                   2.3 \\
Lamp/floor\_lamp          &              0.0 &                 19.3 &&     0.0 &             0.8 &                    20.2 &           1.0 &                  11.3 \\
StorageFurniture/chest   &              1.1 &                  0.3 &&     1.5 &             0.8 &                     0.6 &           1.0 &                   1.0 \\
Table/game\_table         &              0.0 &                  0.0 &&     0.0 &             0.6 &                     0.8 &           7.4 &                   5.6 \\
Laptop/base\_side         &              0.0 &                  0.0 &&     0.0 &             0.0 &                     0.6 &           0.0 &                   0.0 \\
TrashCan/cover           &              5.6 &                  1.3 &&     5.2 &             2.0 &                     1.8 &           4.1 &                   3.4 \\
Chair/chair\_back         &             50.0 &                 28.6 &&    39.6 &            38.8 &                    36.4 &          45.5 &                  42.8 \\
Display/base             &             11.5 &                  8.9 &&     9.3 &            10.9 &                    11.0 &          10.2 &                  10.9 \\
Vase/base                &              0.0 &                  0.0 &&     0.0 &             0.0 &                     0.0 &           0.0 &                   0.0 \\
Bag/paper\_bag            &              7.0 &                  3.6 &&     5.1 &             5.6 &                     4.4 &           5.3 &                   5.0 \\
TrashCan/base            &              7.1 &                  2.0 &&     1.3 &             0.0 &                     0.0 &           1.6 &                   1.6 \\
Display/display\_screen   &             41.5 &                 29.6 &&    35.5 &            41.1 &                    43.1 &          40.4 &                  42.5 \\
Chair/chair\_head         &              0.2 &                  0.2 &&     0.7 &             0.2 &                     0.4 &           0.5 &                   0.5 \\
Keyboard/frame           &              0.1 &                  0.8 &&     0.5 &             4.3 &                     5.2 &           0.5 &                   0.7 \\
Dishwasher/base          &              0.0 &                  0.0 &&     0.0 &             0.0 &                     0.0 &           0.0 &                   0.0 \\
Bed/loft\_bed             &              0.0 &                  1.9 &&     2.4 &             0.0 &                     0.0 &           0.0 &                   0.8 \\
TrashCan/other           &              0.0 &                  0.0 &&     0.0 &             0.0 &                     0.0 &           0.0 &                   0.0 \\
Vase/body                &              0.1 &                  0.4 &&     0.1 &             0.0 &                     0.0 &           0.1 &                   0.3 \\
Microwave/base           &              0.0 &                  0.0 &&     0.0 &             0.0 &                     0.0 &           0.0 &                   0.0 \\
Keyboard/key             &              0.0 &                  0.0 &&     0.0 &            14.9 &                    13.9 &           5.9 &                   5.9 \\
\midrule
Mean                     &             12.7 &                  9.5 &&    11.8 &            11.4 &                    11.8 &          11.7 &                  11.9 \\
\bottomrule
\end{tabular}
\end{table}

% --------------------------------------------------------------

\begin{table}[!h]

\caption{middle level mAcc}
\centering
\begin{tabular}{lrrrrrrrr}
\toprule
 &  \multicolumn{2}{c}{Baseline} && \multicolumn{5}{c}{Multi-Task Training (MTT)} \\
 \cmidrule{2-3}
 \cmidrule{5-9}
Class 			  &  	 Mid. &  				Fin. &&  	12 &  		123-coa. &  		123-coa.\,ens. &  	  123-fin. &  123-fin.\,ens. \\
\midrule
Microwave/body           &              2.1 &                  9.8 &&     6.8 &             6.7 &                     8.6 &          11.6 &                  13.6 \\
Laptop/screen\_side       &             19.2 &                 29.6 &&    12.2 &            30.2 &                    30.7 &          19.4 &                  20.3 \\
Bag/luggage              &             49.0 &                  0.0 &&     3.9 &             0.0 &                     0.0 &           0.0 &                   0.0 \\
StorageFurniture/cabinet &             48.1 &                 43.7 &&    43.7 &            63.0 &                    63.9 &          44.3 &                  46.7 \\
Bed/regular\_bed          &             64.0 &                 39.1 &&    56.2 &            47.3 &                    50.0 &          64.3 &                  63.5 \\
Table/desk               &             21.5 &                  9.1 &&    25.1 &            13.0 &                     8.8 &          29.3 &                  21.0 \\
Table/regular\_table      &             65.8 &                 52.5 &&    63.3 &            64.8 &                    64.8 &          61.3 &                  64.6 \\
Chair/chair\_base         &             80.8 &                 76.9 &&    76.6 &            58.9 &                    54.3 &          64.4 &                  58.4 \\
Lamp/table\_lamp          &             36.2 &                 47.7 &&    54.8 &            26.5 &                    30.8 &          35.6 &                  39.4 \\
Dishwasher/body          &              0.0 &                  0.4 &&     0.0 &             0.4 &                     0.5 &           0.0 &                   0.0 \\
TrashCan/outside\_frame   &              0.0 &                  0.0 &&     1.9 &             0.0 &                     0.0 &           0.0 &                   0.0 \\
Chair/chair\_arm          &             55.3 &                 54.6 &&    54.9 &            41.9 &                    43.8 &          44.5 &                  46.4 \\
Bed/bunk\_bed             &              4.9 &                  2.3 &&    20.5 &             3.8 &                     5.1 &           8.7 &                   6.0 \\
Chair/chair\_seat         &             76.9 &                 69.8 &&    78.5 &            60.0 &                    54.5 &          65.0 &                  61.1 \\
TrashCan/container       &             48.5 &                 24.5 &&    39.1 &            22.7 &                    23.4 &          35.0 &                  35.9 \\
Vase/containing\_things   &              4.2 &                  6.3 &&     9.3 &            11.3 &                    11.8 &           5.6 &                   6.2 \\
Bag/hand\_or\_shoulder\_bag &             16.3 &                 18.3 &&    18.0 &            30.3 &                    29.0 &          18.0 &                  18.4 \\
Lamp/floor\_lamp          &              0.0 &                 51.2 &&     0.0 &             0.9 &                    41.2 &           1.2 &                  47.7 \\
StorageFurniture/chest   &              4.1 &                  1.2 &&    10.1 &             5.0 &                     2.6 &           9.8 &                   6.6 \\
Table/game\_table         &              0.0 &                  0.0 &&     0.0 &             1.3 &                     1.6 &          32.4 &                  15.0 \\
Laptop/base\_side         &              0.0 &                  0.0 &&     0.0 &             0.0 &                     0.9 &           0.0 &                   0.0 \\
TrashCan/cover           &              8.0 &                  1.8 &&     9.9 &             2.3 &                     2.0 &           7.3 &                   5.8 \\
Chair/chair\_back         &             65.3 &                 39.8 &&    55.7 &            48.2 &                    45.8 &          53.7 &                  51.6 \\
Display/base             &             40.6 &                 33.1 &&    52.5 &            48.9 &                    47.4 &          59.6 &                  57.8 \\
Vase/base                &              0.0 &                  0.0 &&     0.0 &             0.0 &                     0.0 &           0.0 &                   0.0 \\
Bag/paper\_bag            &             46.3 &                 29.0 &&    28.0 &            24.5 &                    28.2 &          44.8 &                  45.8 \\
TrashCan/base            &             10.7 &                  6.3 &&     4.7 &             0.0 &                     0.0 &           6.7 &                   6.3 \\
Display/display\_screen   &             64.0 &                 53.6 &&    58.2 &            53.7 &                    53.9 &          61.6 &                  64.1 \\
Chair/chair\_head         &              1.5 &                  3.9 &&    10.7 &             2.4 &                     4.9 &           2.4 &                   2.9 \\
Keyboard/frame           &              0.3 &                  2.8 &&     0.7 &             6.6 &                     9.1 &           1.4 &                   1.7 \\
Dishwasher/base          &              0.0 &                  0.0 &&     0.0 &             0.0 &                     0.0 &           0.0 &                   0.0 \\
Bed/loft\_bed             &              0.0 &                  4.4 &&     3.0 &             0.0 &                     0.0 &           0.0 &                   1.4 \\
TrashCan/other           &              0.0 &                  0.0 &&     0.0 &             0.0 &                     0.0 &           0.0 &                   0.0 \\
Vase/body                &              0.3 &                  4.5 &&     0.3 &             0.0 &                     0.0 &           0.7 &                   1.5 \\
Microwave/base           &              0.0 &                  0.0 &&     0.0 &             0.0 &                     0.0 &           0.0 &                   0.0 \\
Keyboard/key             &              0.0 &                  0.0 &&     0.0 &            26.1 &                    27.5 &           8.7 &                   8.7 \\
\midrule
Mean                     &             57.9 &                 47.1 &&    53.5 &            56.2 &                    56.1 &          52.6 &                  53.5 \\
\bottomrule
\end{tabular}
\end{table}

% --------------------------------------------------------------

\begin{table}[!h]
\caption{fine level mIoU}
\centering
\begin{tabular}{lrrrrr}
\toprule
 &  \multicolumn{1}{c}{Baseline} & \multicolumn{4}{c}{Multi-Task Training (MTT)} \\
 \cmidrule{3-6}
Class 			  &  	 Fin. &  	123-coa. &  		123-coa.\,ens. &  	  123-fin. &  123-fin.\,ens. \\
\midrule
Bowl/container                 &            0.0 &             4.4 &                     0.0 &           0.0 &                   0.0 \\
Lamp/lamp\_unit                 &           19.3 &            20.1 &                     2.2 &          11.3 &                   4.7 \\
Laptop/screen                  &            1.7 &             2.8 &                     2.8 &          11.5 &                  10.7 \\
StorageFurniture/cabinet\_door  &           15.2 &            19.7 &                    19.9 &           5.9 &                   6.7 \\
Clock/clock\_body               &            0.4 &             0.6 &                     0.0 &           0.0 &                   0.0 \\
Bed/bed\_unit                   &           22.0 &            32.8 &                    32.4 &          33.3 &                  32.8 \\
StorageFurniture/cabinet\_frame &           12.5 &            10.9 &                    11.9 &          11.4 &                  12.2 \\
StorageFurniture/sink          &            1.9 &             5.9 &                     6.2 &           7.8 &                   7.4 \\
Table/drawer\_base              &            4.2 &             4.1 &                     4.7 &           8.1 &                   8.2 \\
StorageFurniture/drawer        &           10.2 &             6.6 &                     6.6 &           9.5 &                   8.9 \\
Table/table\_base               &           21.6 &            25.1 &                    24.8 &          29.2 &                  28.4 \\
Chair/regular\_leg\_base         &           26.9 &            17.9 &                    19.5 &          27.5 &                  28.9 \\
Microwave/frame                &            3.9 &             2.0 &                     2.2 &           4.4 &                   4.3 \\
Chair/arm\_holistic\_frame       &            1.2 &             0.8 &                     0.8 &           0.5 &                   0.6 \\
StorageFurniture/countertop    &           11.3 &            10.4 &                    10.4 &          10.5 &                   9.9 \\
Bed/ladder                     &            0.9 &             1.9 &                     2.0 &           1.9 &                   1.7 \\
Chair/seat\_surface             &           31.9 &            33.3 &                    34.5 &          34.5 &                  35.3 \\
TrashCan/container\_neck        &            9.9 &             8.3 &                     8.6 &          12.5 &                  12.1 \\
Chair/arm\_slant\_bar            &            0.5 &             0.5 &                     0.7 &           0.2 &                   0.2 \\
Chair/other                    &            0.1 &             0.0 &                     0.0 &           0.1 &                   0.4 \\
Chair/armrest\_hard\_surface     &            3.3 &             2.8 &                     3.0 &           5.0 &                   4.8 \\
Chair/star\_leg\_base            &           21.2 &            12.2 &                    12.2 &          16.4 &                  16.5 \\
Lamp/lamp\_body                 &            3.7 &             8.6 &                     5.2 &           7.0 &                   3.5 \\
Table/tabletop                 &           46.3 &            49.8 &                    51.6 &          50.9 &                  52.3 \\
Chair/foot\_base                &            2.5 &             2.2 &                     1.7 &           2.4 &                   2.2 \\
Chair/arm\_connector            &            2.9 &             1.2 &                     0.8 &           0.8 &                   0.6 \\
TrashCan/frame\_vertical\_bar    &            0.0 &             0.0 &                     0.0 &           0.0 &                   0.0 \\
Table/foosball\_table           &            0.0 &             0.9 &                     0.9 &           6.0 &                   7.4 \\
Vase/plant                     &            1.6 &             4.0 &                     3.6 &           1.2 &                   1.1 \\
Laptop/base\_frame              &            0.0 &             0.8 &                     0.0 &           0.0 &                   0.0 \\
Microwave/door                 &            0.5 &             0.7 &                     1.0 &           1.8 &                   1.7 \\
Laptop/keyboard                &            0.0 &             0.0 &                     0.0 &           0.0 &                   0.0 \\
TrashCan/cover\_frame           &            0.0 &             0.0 &                     0.0 &           0.0 &                   0.0 \\
Chair/arm\_horizontal\_bar       &            1.9 &             1.1 &                     1.5 &           2.9 &                   3.1 \\
Chair/back\_surface             &           20.7 &            23.7 &                    24.8 &          26.5 &                  28.1 \\
\bottomrule
\end{tabular}
\end{table}

\begin{table}[!h]
\caption{fine level mIoU}
\centering
\begin{tabular}{lrrrrr}
\toprule
 &  \multicolumn{1}{c}{Baseline} & \multicolumn{4}{c}{Multi-Task Training (MTT)} \\
 \cmidrule{3-6}
Class 			  &  	 Fin. &  	123-coa. &  		123-coa.\,ens. &  	  123-fin. &  123-fin.\,ens. \\
\midrule
Display/foot\_base              &            0.0 &             0.0 &                     0.0 &           0.0 &                   0.0 \\
Chair/back\_frame               &            4.6 &             4.1 &                     4.4 &           6.2 &                   6.7 \\
Chair/pedestal\_base            &            0.0 &             0.0 &                     0.0 &           0.0 &                   0.0 \\
Chair/arm\_vertical\_bar         &            3.6 &             3.6 &                     3.7 &           3.9 &                   4.1 \\
Display/surface\_base           &           10.3 &            12.1 &                    11.8 &          11.4 &                  11.3 \\
Bag/handle                     &            0.2 &             0.3 &                     0.4 &           0.5 &                   0.7 \\
Display/screen                 &           21.3 &            29.5 &                    29.4 &          24.1 &                  24.0 \\
TrashCan/container\_handle      &            0.0 &             0.0 &                     0.0 &           0.0 &                   0.0 \\
StorageFurniture/cabinet\_base  &            6.6 &             8.1 &                     7.7 &           7.8 &                   6.8 \\
StorageFurniture/mirror        &            0.0 &             0.0 &                     0.0 &           0.0 &                   0.0 \\
Chair/surface\_base             &            0.1 &             0.3 &                     0.3 &           1.4 &                   1.2 \\
Keyboard/frame                 &            0.8 &             5.2 &                     4.9 &           0.7 &                   1.2 \\
Chair/seat\_frame               &            6.3 &             6.1 &                     5.9 &           6.9 &                   6.5 \\
Lamp/lamp\_base                 &            3.5 &             1.9 &                     1.3 &           2.1 &                   1.8 \\
StorageFurniture/object        &            0.9 &             3.6 &                     3.5 &           2.9 &                   2.8 \\
Chair/back\_connector           &            3.3 &             2.8 &                     1.5 &           3.9 &                   1.9 \\
Chair/headrest                 &            0.2 &             0.3 &                     0.4 &           0.5 &                   0.5 \\
Dishwasher/surface\_base        &            0.0 &             0.0 &                     0.0 &           0.0 &                   0.0 \\
Microwave/side\_controls        &            0.6 &             0.6 &                     0.3 &           1.4 &                   1.1 \\
Display/frame                  &           11.7 &            16.6 &                    17.0 &          18.9 &                  18.5 \\
TrashCan/container\_basket      &            0.0 &             0.0 &                     0.0 &           0.0 &                   0.0 \\
TrashCan/wheel\_base            &            2.3 &             0.0 &                     0.0 &           1.7 &                   1.9 \\
TrashCan/frame\_holistic        &            0.0 &             0.0 &                     0.0 &           0.0 &                   0.0 \\
Chair/back\_support             &            3.7 &             3.9 &                     4.0 &           4.4 &                   4.4 \\
StorageFurniture/shelf         &           21.2 &            14.3 &                    14.2 &          18.2 &                  18.1 \\
Bag/bag\_body                   &            3.7 &             5.1 &                     5.3 &           5.0 &                   5.0 \\
Laptop/screen\_frame            &            5.6 &            10.2 &                    12.4 &           5.1 &                   5.7 \\
TrashCan/other\_leaf            &            0.0 &             0.0 &                     0.0 &           0.0 &                   0.0 \\
Vase/container                 &            0.4 &             0.0 &                     0.0 &           0.3 &                   0.1 \\
Chair/arm\_sofa\_style           &           10.5 &            11.3 &                    11.6 &          13.6 &                  14.2 \\
Table/hutch                    &            4.0 &             2.0 &                     1.8 &           1.4 &                   1.5 \\
Chair/armrest\_soft\_surface     &            0.3 &             0.8 &                     0.8 &           1.7 &                   1.9 \\
TrashCan/container\_bottom      &            8.8 &             7.2 &                     7.8 &           9.4 &                   9.4 \\
Bed/furniture                  &            1.8 &             0.0 &                     0.0 &           0.8 &                   0.0 \\
TrashCan/cover\_lid             &            1.8 &             2.0 &                     2.0 &           3.3 &                   3.3 \\
StorageFurniture/chest\_base    &            0.4 &             0.6 &                     0.7 &           1.0 &                   1.0 \\
Chair/arm\_writing\_table        &            0.0 &             0.0 &                     0.0 &           0.0 &                   0.0 \\
Dishwasher/frame               &            0.3 &             0.4 &                     0.4 &           0.0 &                   0.0 \\
Dishwasher/door                &            0.2 &             0.0 &                     0.0 &           0.0 &                   0.0 \\
Chair/pillow                   &            0.1 &             0.4 &                     0.4 &           1.2 &                   1.4 \\
Bag/shoulder\_strap             &            1.3 &             2.2 &                     2.3 &           2.3 &                   2.0 \\
TrashCan/container\_box         &           11.2 &             7.9 &                     8.6 &          14.9 &                  15.5 \\
Chair/seat\_support             &            6.1 &             6.5 &                     6.5 &           7.6 &                   7.5 \\
Keyboard/key                   &            0.0 &            13.8 &                    16.1 &           5.9 &                   5.1 \\
\midrule
Mean                           &            5.8 &             6.3 &                     6.1 &           6.7 &                   6.6 \\
\bottomrule
\end{tabular}
\end{table}

% --------------------------------------------------------------

\begin{table}[!h]
\caption{fine level mAcc}
\centering
\begin{tabular}{lrrrrr}
\toprule
 &  \multicolumn{1}{c}{Baseline} & \multicolumn{4}{c}{Multi-Task Training (MTT)} \\
 \cmidrule{3-6}
Class 			  &  	 Fin. &  	123-coa. &  		123-coa.\,ens. &  	  123-fin. &  123-fin.\,ens. \\
\midrule
Bowl/container                 &            0.0 &            10.8 &                     0.0 &           0.0 &                   0.0 \\
Lamp/lamp\_unit                 &           51.2 &            40.7 &                     2.3 &          47.7 &                   7.4 \\
Laptop/screen                  &            2.3 &             3.0 &                     3.0 &          16.7 &                  15.2 \\
StorageFurniture/cabinet\_door  &           18.6 &            26.2 &                    26.9 &           6.5 &                   7.5 \\
Clock/clock\_body               &           12.6 &            24.8 &                     0.0 &           0.9 &                   0.0 \\
Bed/bed\_unit                   &           39.0 &            49.1 &                    49.8 &          63.4 &                  65.8 \\
StorageFurniture/cabinet\_frame &           13.8 &            12.2 &                    13.6 &          12.5 &                  13.5 \\
StorageFurniture/sink          &            5.4 &            41.3 &                    41.3 &          23.9 &                  20.3 \\
Table/drawer\_base              &            8.5 &             7.0 &                     9.5 &          20.7 &                  25.1 \\
StorageFurniture/drawer        &           16.5 &             8.5 &                     8.5 &          14.0 &                  12.8 \\
Table/table\_base               &           34.3 &            51.4 &                    51.3 &          51.7 &                  48.5 \\
Chair/regular\_leg\_base         &           38.4 &            21.1 &                    23.5 &          31.9 &                  34.2 \\
Microwave/frame                &            6.1 &             2.9 &                     3.0 &           7.3 &                   6.7 \\
Chair/arm\_holistic\_frame       &            2.9 &             4.4 &                     3.4 &           1.9 &                   1.5 \\
StorageFurniture/countertop    &           19.5 &            26.7 &                    26.2 &          27.8 &                  25.2 \\
Bed/ladder                     &            2.3 &             5.1 &                     5.6 &           6.0 &                   5.9 \\
Chair/seat\_surface             &           45.9 &            40.2 &                    43.0 &          41.2 &                  43.0 \\
TrashCan/container\_neck        &           18.9 &            25.7 &                    22.1 &          40.9 &                  33.9 \\
Chair/arm\_slant\_bar            &            6.5 &             3.9 &                     3.6 &           0.6 &                   0.6 \\
Chair/other                    &            1.5 &             0.0 &                     0.0 &           1.5 &                   1.5 \\
Chair/armrest\_hard\_surface     &           23.9 &            13.5 &                    11.7 &          15.5 &                  11.8 \\
Chair/star\_leg\_base            &           58.0 &            17.3 &                    17.3 &          22.6 &                  22.7 \\
Lamp/lamp\_body                 &           30.6 &            22.6 &                    23.0 &          24.8 &                  26.8 \\
Table/tabletop                 &           57.5 &            62.0 &                    66.3 &          65.5 &                  68.6 \\
Chair/foot\_base                &           23.4 &            26.9 &                    19.5 &          22.2 &                  17.0 \\
Chair/arm\_connector            &           14.6 &             6.0 &                     2.3 &           3.7 &                   1.6 \\
TrashCan/frame\_vertical\_bar    &            0.0 &             0.0 &                     0.0 &           0.0 &                   0.0 \\
Table/foosball\_table           &            0.0 &             1.9 &                     1.9 &          18.0 &                  27.8 \\
Vase/plant                     &            6.6 &            12.4 &                    12.2 &           6.6 &                   6.6 \\
Laptop/base\_frame              &            0.0 &             1.2 &                     0.0 &           0.0 &                   0.0 \\
Microwave/door                 &            0.6 &             0.8 &                     1.1 &           3.1 &                   2.6 \\
Laptop/keyboard                &            0.0 &             0.0 &                     0.0 &           0.0 &                   0.0 \\
TrashCan/cover\_frame           &            0.0 &             0.0 &                     0.0 &           0.0 &                   0.0 \\
Chair/arm\_horizontal\_bar       &           22.3 &             7.4 &                     7.1 &          16.9 &                  12.6 \\
Chair/back\_surface             &           26.8 &            27.6 &                    29.4 &          30.7 &                  32.9 \\
\bottomrule
\end{tabular}
\end{table}

\begin{table}[!h]
\caption{fine level mAcc}
\centering
\begin{tabular}{lrrrrr}
\toprule
 &  \multicolumn{1}{c}{Baseline} & \multicolumn{4}{c}{Multi-Task Training (MTT)} \\
 \cmidrule{3-6}
Class 			  &  	 Fin. &  	123-coa. &  		123-coa.\,ens. &  	  123-fin. &  123-fin.\,ens. \\
\midrule
Display/foot\_base              &            0.0 &             0.0 &                     0.0 &           0.0 &                   0.0 \\
Chair/back\_frame               &           13.3 &             8.3 &                     8.9 &          12.5 &                  13.5 \\
Chair/pedestal\_base            &            0.0 &             0.0 &                     0.0 &           0.0 &                   0.0 \\
Chair/arm\_vertical\_bar         &           19.7 &            13.9 &                    10.8 &          14.5 &                  12.1 \\
Display/surface\_base           &           33.2 &            47.5 &                    46.0 &          58.0 &                  57.8 \\
Bag/handle                     &            5.9 &            23.0 &                    17.1 &          10.5 &                  10.5 \\
Display/screen                 &           42.4 &            42.6 &                    42.8 &          37.1 &                  37.2 \\
TrashCan/container\_handle      &            0.0 &             0.0 &                     0.0 &           0.0 &                   0.0 \\
StorageFurniture/cabinet\_base  &           15.1 &            33.9 &                    29.5 &          23.7 &                  18.9 \\
StorageFurniture/mirror        &            0.0 &             0.0 &                     0.0 &           0.0 &                   0.0 \\
Chair/surface\_base             &            0.9 &             0.7 &                     0.7 &           2.6 &                   2.0 \\
Keyboard/frame                 &            2.8 &             9.1 &                     7.3 &           1.7 &                   3.1 \\
Chair/seat\_frame               &           31.9 &            26.9 &                    25.9 &          24.9 &                  24.1 \\
Lamp/lamp\_base                 &           34.9 &            15.6 &                    11.7 &          27.4 &                  24.8 \\
StorageFurniture/object        &            1.7 &            44.8 &                    45.5 &          30.1 &                  30.7 \\
Chair/back\_connector           &            7.5 &             6.1 &                     2.6 &           6.7 &                   3.0 \\
Chair/headrest                 &            3.9 &             4.9 &                     4.4 &           2.9 &                   2.4 \\
Dishwasher/surface\_base        &            0.0 &             0.0 &                     0.0 &           0.0 &                   0.0 \\
Microwave/side\_controls        &            1.7 &             6.8 &                     1.7 &           5.1 &                   3.4 \\
Display/frame                  &           23.8 &            23.8 &                    26.0 &          35.8 &                  36.3 \\
TrashCan/container\_basket      &            0.0 &             0.0 &                     0.0 &           0.0 &                   0.0 \\
TrashCan/wheel\_base            &            9.1 &             0.0 &                     0.0 &           9.1 &                   9.1 \\
TrashCan/frame\_holistic        &            0.0 &             0.0 &                     0.0 &           0.0 &                   0.0 \\
Chair/back\_support             &            6.8 &             6.3 &                     6.7 &           9.5 &                   9.8 \\
StorageFurniture/shelf         &           46.2 &            38.1 &                    38.1 &          32.8 &                  32.6 \\
Bag/bag\_body                   &           27.7 &            20.9 &                    21.4 &          43.3 &                  43.9 \\
Laptop/screen\_frame            &           23.5 &            24.8 &                    24.4 &          11.9 &                  12.2 \\
TrashCan/other\_leaf            &            0.0 &             0.0 &                     0.0 &           0.0 &                   0.0 \\
Vase/container                 &            4.5 &             0.0 &                     0.0 &           1.5 &                   0.8 \\
Chair/arm\_sofa\_style           &           40.0 &            32.8 &                    33.7 &          33.9 &                  35.5 \\
Table/hutch                    &           20.6 &            19.5 &                    10.7 &           7.6 &                   5.7 \\
Chair/armrest\_soft\_surface     &            1.8 &             7.6 &                     5.6 &          12.2 &                   9.0 \\
TrashCan/container\_bottom      &           31.0 &            14.7 &                    16.1 &          39.7 &                  39.5 \\
Bed/furniture                  &            4.3 &             0.0 &                     0.0 &           1.4 &                   0.0 \\
TrashCan/cover\_lid             &            2.0 &             2.2 &                     2.2 &           5.6 &                   5.5 \\
StorageFurniture/chest\_base    &            2.1 &             3.9 &                     5.5 &          11.0 &                  11.5 \\
Chair/arm\_writing\_table        &            NaN &             NaN &                     NaN &           NaN &                   NaN \\
Dishwasher/frame               &            0.6 &             1.3 &                     1.2 &           0.0 &                   0.0 \\
Dishwasher/door                &            0.2 &             0.0 &                     0.0 &           0.0 &                   0.0 \\
Chair/pillow                   &            0.8 &            14.7 &                    13.3 &          31.4 &                  26.0 \\
Bag/shoulder\_strap             &           18.3 &            28.9 &                    29.1 &          18.4 &                  17.6 \\
TrashCan/container\_box         &           11.7 &             8.1 &                     8.9 &          16.2 &                  17.3 \\
Chair/seat\_support             &           31.6 &            13.9 &                    12.8 &          24.2 &                  22.2 \\
Keyboard/key                   &            0.0 &            27.5 &                    26.1 &           8.7 &                   7.2 \\
\midrule
Mean                           &           31.0 &            32.5 &                    33.8 &          34.7 &                  35.6 \\
\bottomrule
\end{tabular}
\end{table}

\paragraph{Qualitative semantic labeling results}
\label{supsec:results:semantic-segmentation-qualitative}

% \VI{DONE: add figure with more visualizations}
%  6. Несколько дополнительных результатов работы алгоритма (нет) (наподобие рисунка 4 основной статьи)

\begin{figure}[!t]
\label{fig:semantic_experiments}
\centering
\includegraphics[width=\textwidth]{images/semantic_experiments.pdf}
\caption{Qualitative semantic labeling results}
\end{figure}

\subsection{Hierarchical semantic segmentation}
\label{supsec:results:hierarchical-segmentation}

% \AN{3 tables with class/part-wise results on hierarchical semantic segmentation for 3 different levels of detail}
\begin{table}[!htb]
\caption{results of the models on Hierarchical Segmentation task on coarse level of detail}
\begin{tabular}{lrr}
\toprule
{} &  balanced\_accuracy\_score &  iou \\
\midrule
Microwave/microwave                &                      3.0 &  1.9 \\
Bowl/bowl                          &                      0.0 &  0.0 \\
Display/display                    &                     55.0 & 38.4 \\
Faucet/faucet                      &                      0.0 &  0.0 \\
Lamp/lamp                          &                     31.3 &  9.3 \\
Laptop/laptop                      &                     11.7 &  3.0 \\
Bag/bag                            &                     29.6 &  6.7 \\
StorageFurniture/storage\_furniture &                     59.7 & 49.6 \\
Clock/clock                        &                      5.6 &  0.1 \\
Bed/bed                            &                     49.1 & 31.9 \\
Table/table                        &                     69.9 & 42.5 \\
Chair/chair                        &                     55.7 & 44.0 \\
Hat/hat                            &                      --- &  --- \\
Dishwasher/dishwasher              &                      0.0 &  0.0 \\
TrashCan/trash\_can                 &                     29.7 & 21.8 \\
Vase/pot                           &                      0.5 &  0.3 \\
Bottle/bottle                      &                      --- &  --- \\
Keyboard/keyboard                  &                     18.5 &  3.5 \\
\bottomrule
\end{tabular}
\end{table}

\begin{table}[!htb]
\caption{results of the models on Hierarchical Segmentation task on middle level of detail}
\begin{tabular}{lrr}
\toprule
{} &  balanced\_accuracy\_score &  iou \\
\midrule
Microwave/body           &                      3.2 &  2.0 \\
Bowl/container           &                      0.0 &  0.0 \\
Display/accessories      &                      --- &  0.0 \\
Faucet/normal\_faucet     &                      0.0 &  0.0 \\
Lamp/wall\_lamp           &                      0.0 &  0.0 \\
Laptop/screen\_side       &                     20.8 &  4.1 \\
Bag/luggage              &                      0.0 &  0.0 \\
StorageFurniture/cabinet &                     60.2 & 50.0 \\
Clock/normal\_clock       &                      0.0 &  0.0 \\
Bed/regular\_bed          &                     48.7 & 30.3 \\
Table/desk               &                      6.5 &  3.7 \\
Table/regular\_table      &                     71.2 & 42.5 \\
Chair/chair\_base         &                     45.9 & 37.7 \\
Hat/normal\_hat           &                      --- &  --- \\
Lamp/table\_lamp          &                     31.7 &  9.5 \\
Dishwasher/body          &                      0.0 &  0.0 \\
TrashCan/outside\_frame   &                      0.0 &  0.0 \\
Chair/chair\_arm          &                     29.4 & 12.8 \\
Bed/bunk\_bed             &                      0.8 &  0.8 \\
Chair/chair\_seat         &                     46.0 & 32.8 \\
TrashCan/container       &                     32.1 & 23.0 \\
Vase/containing\_things   &                      0.4 &  0.3 \\
Bottle/normal\_bottle     &                      --- &  --- \\
Bag/hand\_or\_shoulder\_bag &                     12.4 &  1.5 \\
Lamp/floor\_lamp          &                      0.0 &  0.0 \\
StorageFurniture/chest   &                      3.0 &  0.6 \\
Table/game\_table         &                      2.6 &  1.1 \\
Laptop/base\_side         &                      0.0 &  0.0 \\
TrashCan/cover           &                      4.4 &  2.8 \\
Chair/chair\_back         &                     40.1 & 31.5 \\
Display/base             &                     27.3 & 12.0 \\
Laptop/connector         &                      0.0 &  0.0 \\
Vase/base                &                      0.0 &  0.0 \\
Bag/paper\_bag            &                     22.2 &  5.7 \\
Keyboard/other           &                      --- &  --- \\
Lamp/street\_lamp         &                      --- &  0.0 \\
TrashCan/base            &                      0.8 &  0.4 \\
Display/display\_screen   &                     55.8 & 40.3 \\
Chair/chair\_head         &                      6.3 &  2.5 \\
Keyboard/frame           &                     11.8 &  2.6 \\
Dishwasher/base          &                      0.0 &  0.0 \\
Bag/briefcase            &                      --- &  --- \\
Bed/loft\_bed             &                     14.3 &  6.1 \\
Bowl/bottom              &                      --- &  --- \\
Keyboard/tilt\_leg        &                      0.0 &  0.0 \\
TrashCan/other           &                      0.0 &  0.0 \\
Vase/body                &                      0.8 &  0.3 \\
Microwave/base           &                      0.0 &  0.0 \\
Table/picnic\_table       &                      0.0 &  0.0 \\
Keyboard/key             &                     13.0 &  1.5 \\
\bottomrule
\end{tabular}
\end{table}

\paragraph{Qualitative hierarchical semantic segmentation results}
\label{supsec:results:hierarchical-segmentation-qualitative}

% \VI{DONE: add figure with more visualizations}
%  6. Несколько дополнительных результатов работы алгоритма (нет) (наподобие рисунка 4 основной статьи)

\begin{figure}[!t]
\label{fig:hierarchy_experiments}
\centering
\includegraphics[width=\textwidth]{images/hierarchy_experiments.pdf}
\caption{Qualitative hierarchical semantic segmentation results}
\end{figure}

\subsection{Semantic instance segmentation}
\label{supsec:results:instance-segmentation}

% \AN{3 tables with part-wise results on semantic instance segmentation for 3 different levels of detail}

\begin{table}[!htb]
\caption{results of the models on Instance Segmentation task, original model and with background push}
% \resizebox{\textwidth}{!}{%
\begin{tabular}{l|lll|lll}
model & \multicolumn{3}{c}{InstSeg} & \multicolumn{3}{c}{InstSeg bg push} \\
classes & IoU & (AP@50) & recall (@50) & IoU & (AP@50) & recall (@50) \\
\hline
Microwave & \textbf{90.93\%} & \textbf{87.50\%} & \textbf{33.33\%} & 80.59\% & 75.00\% & 28.57\% \\
Display & \textbf{76.15\%} & \textbf{64.62\%} & 29.58\% & 73.59\% & 64.00\% & \textbf{33.80\%} \\
Lamp & 65.29\% & 75.00\% & \textbf{34.62\%} & \textbf{70.64\%} & \textbf{77.78\%} & 26.92\% \\
Laptop & \textbf{50.44\%} & \textbf{100.00\%} & \textbf{9.09\%} & NaN & 0.00\% & 0.00\% \\
Bag & 89.19\% & \textbf{100.00\%} & \textbf{33.33\%} & \textbf{91.70\%} & 75.00\% & 27.27\% \\
Storage & \textbf{82.01\%} & 71.71\% & 37.30\% & 81.44\% & \textbf{74.70\%} & \textbf{38.10\%} \\
Bed & \textbf{79.55\%} & 62.86\% & 63.77\% & 78.38\% & \textbf{74.29\%} & \textbf{75.36\%} \\
Table & 77.34\% & 77.10\% & 42.49\% & \textbf{80.35\%} & \textbf{81.37\%} & \textbf{46.20\%} \\
Chair & 82.88\% & 82.14\% & 30.50\% & \textbf{86.01\%} & \textbf{86.79\%} & \textbf{32.23\%} \\
Dishwasher & 71.32\% & 100.00\% & 66.67\% & \textbf{72.66\%} & \textbf{100.00\%} & \textbf{66.67\%} \\
TrashCan & 87.22\% & \textbf{86.18\%} & \textbf{53.27\%} & \textbf{89.88\%} & 85.12\% & 51.76\% \\
Vase & \textbf{90.83\%} & 100.00\% & 33.33\% & 80.89\% & \textbf{100.00\%} & \textbf{55.56\%} \\
\hline
mIoU / mAP & 78.60\% & \textbf{83.93\%} & 35.94\% & \textbf{80.56\%} & 74.50\% & \textbf{37.11\%}
\end{tabular}%
\label{tab:lod1instsegresults}
% }
\end{table}

\begin{table}[!htb]
\caption{Instance Segmentation results on middle level of detail}
\begin{tabular}{lrrrr}
\toprule
{} &  iou &  precision &  recall &  num\_instances \\
\midrule
Microwave/body           & 74.4 &       45.5 &    23.8 &             21 \\
Laptop/screen\_side       & 99.0 &      100.0 &    50.0 &              2 \\
StorageFurniture/cabinet &  --- &        --- &     0.0 &              1 \\
Bed/regular\_bed          &  --- &        --- &     0.0 &              2 \\
Table/desk               &  --- &        0.0 &     0.0 &             11 \\
Table/regular\_table      &  --- &        --- &     0.0 &              4 \\
Chair/chair\_base         & 78.0 &       68.9 &    34.9 &            496 \\
Lamp/table\_lamp          & 76.0 &      100.0 &   100.0 &              2 \\
Dishwasher/body          & 72.3 &       49.2 &    46.4 &             69 \\
TrashCan/outside\_frame   & 52.5 &       26.7 &     3.4 &            118 \\
Chair/chair\_arm          & 76.0 &       61.7 &    32.3 &            539 \\
Bed/bunk\_bed             & 76.5 &       70.7 &    21.3 &            746 \\
TrashCan/container       & 69.8 &       75.0 &    46.2 &             26 \\
Vase/containing\_things   & 71.6 &       66.7 &    66.7 &              6 \\
Bag/hand\_or\_shoulder\_bag & 70.6 &      100.0 &    57.1 &              7 \\
Lamp/floor\_lamp          & 59.1 &       11.8 &     2.6 &            421 \\
StorageFurniture/chest   &  --- &        0.0 &     0.0 &             21 \\
Table/game\_table         & 71.9 &       67.8 &    20.9 &            748 \\
Laptop/base\_side         & 82.6 &       82.4 &    42.6 &            197 \\
TrashCan/cover           & 62.6 &       27.3 &    33.3 &              9 \\
Display/base             &  --- &        --- &     0.0 &             27 \\
Vase/base                &  --- &        --- &     0.0 &              1 \\
Bag/paper\_bag            & 87.1 &       50.0 &     2.5 &             40 \\
TrashCan/base            &  --- &        --- &     0.0 &              3 \\
Display/display\_screen   &  --- &        --- &     0.0 &              7 \\
Chair/chair\_head         & 64.1 &       50.0 &     5.4 &             37 \\
Keyboard/frame           & 73.6 &       62.4 &    17.1 &            735 \\
Dishwasher/base          &  --- &        0.0 &     0.0 &            106 \\
Bed/loft\_bed             &  --- &        --- &     0.0 &              1 \\
TrashCan/other           &  --- &        0.0 &     0.0 &              2 \\
Vase/body                & 75.1 &       61.1 &    33.3 &             33 \\
\midrule
Mean                     & 70.5 &       54.2 &    19.7 &             93 \\
\bottomrule
\end{tabular}
\end{table}

\begin{table}[!htb]
\caption{Instance Segmentation results on fine level of detail}
\begin{tabular}{lrrrr}
\toprule
{} &  iou &  precision &  recall &  num\_instances \\
\midrule
Bowl/container                 &  --- &        --- &     0.0 &              1 \\
Lamp/lamp\_unit                 & 67.3 &       50.0 &    50.0 &              2 \\
Clock/clock\_body               & 82.5 &       52.9 &    34.6 &             26 \\
Bed/bed\_unit                   & 51.2 &      100.0 &    11.1 &              9 \\
StorageFurniture/cabinet\_frame &  --- &        --- &     0.0 &              2 \\
StorageFurniture/sink          & 61.7 &       22.8 &     6.8 &            308 \\
Table/drawer\_base              & 99.5 &      100.0 &   100.0 &              2 \\
StorageFurniture/drawer        & 74.8 &       63.2 &    62.3 &             69 \\
Table/table\_base               & 69.0 &       37.5 &    17.6 &            495 \\
Chair/regular\_leg\_base         & 53.6 &       66.7 &    26.1 &             23 \\
Microwave/frame                & 55.9 &       21.7 &     8.5 &            118 \\
Chair/arm\_holistic\_frame       &  --- &        --- &     0.0 &              1 \\
StorageFurniture/countertop    & 57.6 &       26.8 &     5.9 &            188 \\
Bed/ladder                     & 66.3 &       46.1 &    21.9 &            538 \\
Chair/seat\_surface             & 70.7 &       60.3 &    18.2 &            693 \\
Chair/arm\_slant\_bar            & 67.9 &       26.7 &    19.0 &             21 \\
Chair/other                    &  --- &        --- &     0.0 &              1 \\
Chair/armrest\_hard\_surface     &  --- &        --- &     0.0 &              2 \\
Chair/star\_leg\_base            &  --- &        0.0 &     0.0 &              3 \\
Lamp/lamp\_body                 & 54.5 &        8.3 &     2.7 &             37 \\
Table/tabletop                 &  --- &        0.0 &     0.0 &             43 \\
Chair/foot\_base                &  --- &        --- &     0.0 &             14 \\
Chair/arm\_connector            & 70.7 &       58.4 &    21.9 &            744 \\
TrashCan/frame\_vertical\_bar    & 65.7 &       46.2 &     7.2 &             83 \\
Table/foosball\_table           & 50.0 &       50.0 &     7.3 &             41 \\
Vase/plant                     & 84.4 &       66.7 &    20.0 &             10 \\
Laptop/base\_frame              & 67.2 &       30.6 &     6.4 &            173 \\
Microwave/door                 & 65.3 &       55.6 &    24.0 &            229 \\
TrashCan/cover\_frame           & 59.0 &       50.0 &     9.1 &             22 \\
Display/foot\_base              &  --- &        --- &     0.0 &              3 \\
Chair/back\_frame               & 74.2 &       63.0 &    35.8 &            537 \\
Display/surface\_base           & 56.7 &       40.0 &     5.1 &             79 \\
Bag/handle                     & 70.8 &       50.0 &     5.8 &            104 \\
Display/screen                 & 58.8 &       66.7 &    50.0 &              4 \\
TrashCan/container\_handle      &  --- &        --- &     0.0 &              1 \\
StorageFurniture/cabinet\_base  &  --- &        --- &     0.0 &              2 \\
Keyboard/frame                 & 71.2 &       62.5 &    55.6 &              9 \\
Chair/seat\_frame               &  --- &        --- &     0.0 &              7 \\
\bottomrule
\end{tabular}
\end{table}

\begin{table}[!htb]
\caption{Instance Segmentation results on fine level of detail}
\begin{tabular}{lrrrr}
\toprule
{} &  iou &  precision &  recall &  num\_instances \\
\midrule

Lamp/lamp\_base                 &  --- &        --- &     0.0 &             20 \\
StorageFurniture/object        &  --- &        --- &     0.0 &              5 \\
Chair/back\_connector           &  --- &        --- &     0.0 &              5 \\
Chair/headrest                 & 75.0 &       12.5 &     2.0 &            100 \\
Microwave/side\_controls        & 69.2 &       61.5 &    18.9 &            734 \\
Display/frame                  &  --- &        --- &     0.0 &              1 \\
TrashCan/wheel\_base            & 56.0 &       16.0 &     2.7 &            295 \\
TrashCan/frame\_holistic        &  --- &        --- &     0.0 &              2 \\
Chair/back\_support             & 71.3 &       50.0 &   100.0 &              1 \\
StorageFurniture/shelf         &  --- &        --- &     0.0 &              1 \\
Bag/bag\_body                   & 75.5 &      100.0 &    50.0 &              2 \\
Laptop/screen\_frame            & 64.9 &       26.7 &     2.1 &            193 \\
TrashCan/other\_leaf            &  --- &        0.0 &     0.0 &            105 \\
Vase/container                 &  --- &        --- &     0.0 &              1 \\
Chair/arm\_sofa\_style           &  --- &        --- &     0.0 &             24 \\
Bed/furniture                  & 56.7 &       49.2 &    20.4 &            142 \\
TrashCan/cover\_lid             &  --- &        0.0 &     0.0 &              1 \\
StorageFurniture/chest\_base    &  --- &        --- &     0.0 &              6 \\
Chair/arm\_writing\_table        & 53.3 &       11.1 &     1.3 &            158 \\
Dishwasher/frame               &  --- &        --- &     0.0 &              2 \\
Dishwasher/door                &  --- &        --- &     0.0 &             11 \\
Chair/pillow                   & 57.8 &       66.7 &    18.2 &             11 \\
Bag/shoulder\_strap             &  --- &        --- &     0.0 &              1 \\
TrashCan/container\_box         &  --- &        --- &     0.0 &              3 \\
Chair/seat\_support             &  --- &        --- &     0.0 &              9 \\
Keyboard/key                   & 61.1 &        7.7 &     0.8 &            242 \\
\midrule
Mean                           & 64.7 &       41.4 &    11.8 &             64 \\
\bottomrule
\end{tabular}
\end{table}
%  6. Несколько дополнительных результатов работы алгоритма (нет) (наподобие рисунка 4 основной статьи)

\paragraph{Qualitative semantic instance segmentation results}
\label{supsec:results:instance-segmentation-qualitative}

% \VI{DONE: add figure with more visualizations}

\begin{figure}[!t]
\label{fig:instance_experiments}
\centering
\includegraphics[width=\textwidth]{images/instance_experiments.pdf}
\caption{Qualitative semantic instance segmentation results}
\end{figure}
